# Supplementary material for: Computational inverse method for constructing spaces of quantum models from wave functions
Source: arXiv:1802.01590 ancillary file (2018-07-12)
Supplement: Supplementary file 1 [file suppMaterial.pdf]

## Supplemental Material

## I. DEGENERATE EIGENSTATE-TO-HAMILTONIAN CONSTRUCTION

Here we present Degenerate Eigenstate-to-Hamiltonian Construction (DEHC), a generalization of the EHC method for constructing Hamiltonians with multiple target states as degenerate energy eigenstates.

In this formulation, the input is a set of Hermitian operators $\{\hat{h}_a\}_{a=1}^{d_T}$ and $M$ target states $|\psi_{T,1}\rangle, \ldots, |\psi_{T,M}\rangle$. However, first, we describe the method by considering using a target density matrix $\hat{\rho}_T$ as input rather than the set of target states. Then, we discuss how the density matrix can be defined in terms of our target states to achieve the desired result. Using the density matrix $\hat{\rho}_T$, we can define the density matrix quantum covariance matrix (DQCM), a generalization of the QCM, whose matrix elements are

$$(D_T)_{ab} = \langle \hat{h}_a \hat{h}_b \rangle_T - \langle \hat{h}_a \rangle_T \langle \hat{h}_b \rangle_T \tag{1}$$

where the expectation values are defined by a trace over the target density matrix: $\langle \hat{\mathcal{O}} \rangle_T \equiv \mathrm{tr}\left(\hat{\rho}_T \hat{\mathcal{O}}\right)$. The $D_T$ matrix, like the QCM $C_T$ discussed in the paper, is Hermitian and positive semi-definite.

Despite the apparent similarity of the DQCM to the QCM, the null space of the DQCM has a different interpretation than that of the QCM. To see this, consider a vector of coupling constants $J_a$ in the null space of $D_T$. This vector corresponds to a Hamiltonian $\hat{H} = \sum_{a=1}^{d_T} J_a \hat{h}_a$ with energy eigenstates $|n\rangle$. Let us express the target density matrix in terms of the eigenstates of $\hat{H}$ so that $\hat{\rho}_T = \sum_{m,n} \rho_{mn} |m\rangle \langle n|$, where the normalization is such that $\mathrm{tr}\left(\hat{\rho}_T\right) = \sum_n p_n = 1$ where $p_n \equiv \rho_{nn} \geq 0$. Since $J_a$ is in the null space of $D_T$, the Hamiltonian $\hat{H}$ has zero energy variance, which can be expressed as

$$\begin{aligned} \sigma_T^2 &= \mathrm{tr}\left(\hat{\rho}_T \hat{H}^2\right) - \mathrm{tr}\left(\hat{\rho}_T \hat{H}\right)^2 \\ &= \sum_n p_n E_n^2 - \left(\sum_n p_n E_n\right)^2 \\ &= \sum_n p_n E_n \left(E_n - \sum_m p_m E_m\right) = 0 \end{aligned} \tag{2}$$

where the $E_n$ are the energy eigenvalues of $|n\rangle$. For Eq. (2) to be satisfied, each term in the summation needs to be zero, which occurs when $E_n = \langle \hat{H} \rangle_T = \sum_m p_m E_m =$ constant for all

$n$ for which $p_n > 0$. This means that the states $|n\rangle$ with $p_n > 0$ in the density matrix are degenerate eigenstates of the Hamiltonian $\hat{H}$. Therefore, it becomes apparent that the null space of the DQCM corresponds to a space of Hamiltonians that contain multiple target wave functions as degenerate energy eigenstates. Finally, we can invert this perspective, and use a set of target states $|\psi_{T,1}\rangle, \ldots, |\psi_{T,M}\rangle$ to define our target density matrix $\hat{\rho}_T = \sum_{m=1}^{M} p_m |\psi_{T,m}\rangle\langle\psi_{T,m}|$ with $p_m > 0$ and $\sum_{m=1}^{M} p_m = 1$. Note that in DEHC the target states need not be orthogonal to one another, only linearly independent, and that the choice of $p_m$ does not affect the null space of the DQCM. We always used $p_1 = \cdots = p_M = 1/M$ in our calculations.

When we compute the DQCM, we find it useful to break up the calculation into individual calculations for each target state. From Eq. (1) and our definition for the target density matrix, the DQCM can be expressed in terms of the target states $|\psi_{T,m}\rangle$ as follows

$$(D_T)_{a,b} = \sum_{m=1}^{M} p_m \langle \hat{h}_a \hat{h}_b \rangle_{T,m} - \left( \sum_{m=1}^{M} p_m \langle \hat{h}_a \rangle_{T,m} \right) \left( \sum_{m'=1}^{M} p_{m'} \langle \hat{h}_b \rangle_{T,m'} \right) \quad (3)$$

where $\langle \hat{\mathcal{O}} \rangle_{T,m} \equiv \langle \psi_{T,m} | \hat{\mathcal{O}} | \psi_{T,m} \rangle / \langle \psi_{T,m} | \psi_{T,m} \rangle$ is an expectation value for a single target state $|\psi_{T,m}\rangle$. We emphasize that calculating the DQCM with Eq. (3) is different than calculating many QCMs $C_{T,1}, \ldots, C_{T,M}$. Moreover, the intersection of the null spaces of $C_{T,1}, \ldots, C_{T,M}$ correspond to Hamiltonians with the target states as simultaneous eigenstates, but not necessarily degenerate eigenstates. Numerically, one can compute the DQCM with matrix product states and variational Monte Carlo, just as described in the main paper.

## II. UNIFORM FRUSTRATED ISING STATE EIGENSTATE SPACE

For the uniform frustrated Ising (UFI) state $|\psi_{UFI}\rangle$, which is a uniform superposition of the ground states of a frustrated antiferromagnetic Ising model on a two-leg triangular ladder, we found a 21 dimensional space of Hamiltonians with $|\psi_{UFI}\rangle$ as an eigenstate using EHC. In the main paper, we discussed three of these Hamiltonians, $\hat{H}_I$, $\hat{H}^{(1)}_{UFI}$ and $\hat{H}^{(2)}_{UFI}$. Here we present additional operators that we found.

We were able to identify the following operators in the target space we considered:

$$\sum_{i=1}^{N} \sigma_i^z + \frac{1}{3}\sigma_i^z\sigma_{i+1}^z\sigma_{i+2}^z$$

$$\sum_{i=1}^{N} \sigma_i^z - \frac{1}{2}\sigma_i^z\sigma_{i+1}^z\sigma_{i+3}^z - \frac{1}{2}\sigma_i^z\sigma_{i+2}^z\sigma_{i+3}^z$$

$$\sum_{i=1}^{N} \sigma_i^z - \sigma_i^x\sigma_{i+2}^z + \sigma_i^z\sigma_{i+2}^x - \sigma_i^z\sigma_{i+2}^z\sigma_{i+3}^z$$

$$\sum_{i=1}^{N} \sigma_i^x + \sigma_i^x\sigma_{i+1}^z\sigma_{i+2}^z + \sigma_i^x\sigma_{i+1}^z\sigma_{i+3}^z + \sigma_i^x\sigma_{i+2}^z\sigma_{i+3}^z$$

$$\sum_{i=1}^{N} \sigma_i^x + \sigma_i^z\sigma_{i+1}^z\sigma_{i+2}^x + \sigma_i^z\sigma_{i+1}^z\sigma_{i+3}^x + \sigma_i^z\sigma_{i+2}^z\sigma_{i+3}^x$$

$$\sum_{i=1}^{N} \sigma_i^x\sigma_{i+1}^z\sigma_{i+3}^x + \sigma_i^y\sigma_{i+1}^z\sigma_{i+3}^y + \sigma_i^x\sigma_{i+2}^z\sigma_{i+3}^x + \sigma_i^y\sigma_{i+2}^z\sigma_{i+3}^y$$

$$\sum_{i=1}^{N} \sigma_i^x\sigma_{i+1}^x\sigma_{i+2}^x - \sigma_i^x\sigma_{i+1}^y\sigma_{i+2}^y - \sigma_i^y\sigma_{i+1}^x\sigma_{i+2}^y - \sigma_i^y\sigma_{i+1}^y\sigma_{i+2}^x$$

$$\sum_{i=1}^{N} \sigma_i^x\sigma_{i+1}^x\sigma_{i+3}^z - \sigma_i^y\sigma_{i+1}^y\sigma_{i+3}^z - \sigma_i^z\sigma_{i+2}^x\sigma_{i+3}^x + \sigma_i^z\sigma_{i+2}^y\sigma_{i+3}^y$$

$$\sum_{i=1}^{N} \sigma_i^x\sigma_{i+1}^x\sigma_{i+2}^z - \sigma_i^y\sigma_{i+1}^y\sigma_{i+2}^z - \sigma_i^z\sigma_{i+1}^x\sigma_{i+2}^x - \sigma_i^z\sigma_{i+1}^y\sigma_{i+2}^y.$$

The UFI state is a zero energy eigenstate of each of these operators and any linear combination of them. These operators, as well as $\hat{H}_{UFI}^{(1)}$ and $\hat{H}_{UFI}^{(2)}$, seem to enforce constraints on the spin configurations making up the UFI state. This might be related to the up-up-down constraint used to construct the state. We note that at least some of the Hamiltonians of the form $H_I + J_1\hat{H}_{UFI}^{(1)} + J_2\hat{H}_{UFI}^{(2)}$ for non-zero $J_1$ and $J_2$ have $|\psi_{UFI}\rangle$ as a ground states, but we did not exhaustively determine the ground state manifold.

## III. ADDITIONAL EXAMPLES OF PHASE EXPANSION

Here we present additional results obtained by using EHC and DEHC to construct new parent Hamiltonians with the same ground states as known model Hamiltonians. A summary of these results are shown in Table S1.

| Target state(s) | $d_T$ | Dim. e.s. space | Dim. g.s. manifold |
|---|---|---|---|
| $\left\|\psi_{KC}^{\pm}\right\rangle$ | 210 | 77 | $\geq 22$ |
| $\|\psi_H\rangle$ | 198 | 39 | $\geq 3$ |
| $\left\|\psi_{SD}^{\pm}\right\rangle$ | 198 | 108 | $\geq 36$ |

TABLE S1. A summary of phase expansion results obtained in this work that are not presented in detail in the main paper. Target states and the dimensions of the input target space, the output eigenstate space, and the ground state manifold are listed. Each of these examples were for length $N = 12$ chains. For each of the ground state manifolds, we could only identify a lower bound for its dimensionality.

### A. Kitaev chain ground states

In this section, we discuss our results of using the DEHC method to construct parent Hamiltonians for the ground state of the Kitaev chain model of superconducting spinless fermions: $\hat{H}_{KC} = \sum_{i=1}^{N-1}\left(-c_i^\dagger c_{i+1} + c_i c_{i+1} + h.c.\right)$. This Hamiltonian is known to have two zero energy single-particle edge modes and, correspondingly, two degenerate many-body ground states [1]. We specify the two degenerate ground states $\left|\psi_{KC}^{\pm}\right\rangle$ of $\hat{H}_{KC}$ as the target states $|\psi_{T,1}\rangle$ and $|\psi_{T,2}\rangle$ provided as input to DEHC. We obtain matrix product state representations of these states by performing DMRG on a finite size chain of $N = 12$ sites.

The target space of Hamiltonians that we provide as input to DEHC is the $d_T$-dimensional space spanned by all possible one and two-site operators of the form

$$n_i, \quad (c_i^\dagger c_j + h.c.), \quad (c_i c_j + h.c.), \quad n_i n_j \tag{4}$$

where $d_T = N + 3\binom{N}{2} = N + 3N(N-1)/2 = 210$ for the $N = 12$ site chain. By examining the null space of the DQCM matrix, we found that the eigenstate space of Hamiltonians was spanned by 77 operators of four types. Three types of operators we found were

$$\begin{aligned}
\hat{H}_{KC}^{(0,i)} &= \left(-c_i^\dagger c_{i+1} + c_i c_{i+1} + h.c.\right) \\
\hat{H}_{KC}^{(1,i)} &= \frac{1}{2}\left(c_i c_{i+1} + h.c.\right) + n_i n_{i+1} - \frac{1}{2}\left(n_i + n_{i+1}\right) \\
\hat{H}_{KC}^{(2,j)} &= \frac{1}{2}\left(-c_j^\dagger c_{j+2} + c_j c_{j+2} + h.c.\right) - n_{j+1}
\end{aligned} \tag{5}$$

for $1 \leq i \leq N-1$ and $1 \leq j \leq N-2$. There are $N-1 = 11$ operators of type $\hat{H}_{KC}^{(0,i)}$ and $\hat{H}_{KC}^{(1,i)}$

and $N-2=10$ operators of type $\hat{H}_{KC}^{(2,i)}$. The energy eigenvalues of $|\psi_{KC}^{\pm}\rangle$ for $\hat{H}_{KC}^{(0,i)}, \hat{H}_{KC}^{(1,i)}$, and $\hat{H}_{KC}^{(2,j)}$ are $-1, -1/2$, and $-1/2$, respectively. Moreover, we numerically verified that the target states are exact ground states of each of the $\hat{H}_{KC}^{(0,i)}, \hat{H}_{KC}^{(1,i)}$ operators and that $[\hat{H}_{KC}^{(0,i)}, \hat{H}_{KC}^{(1,i)}]=0$. The structure of these operators, i.e., that they involve only local one and two-site operators, is consistent with the fact that the Kitaev chain is frustration-free and that the two degenerate ground states of $\hat{H}_{KC}$ can be expressed as product states over the sites [2].

In addition to the operators presented in Eq. (5), we find non-local operators also contained in the eigenstate space:

$$\hat{H}_{KC}^{(3,k,l)} = \sum_{\delta=0,1} \left( -c_{k+\delta}^{\dagger} c_{l-\delta} + (-1)^{\delta} c_{k+\delta} c_{l-\delta} + h.c. \right) \tag{6}$$

where $1 \leq k \leq N-3$ and $k+3 \leq l \leq N$. There are $(N-2)(N-3)/2 = 45$ of the $\hat{H}_{KC}^{(3,k,l)}$ operators for the $N=12$ chain. Note that these operators, unlike the ones from Eq. (5), are not nearest-neighbor, but can connect sites separated by distances of up to $N/2$. The $|\psi_{KC}^{\pm}\rangle$ states are zero energy eigenstates of these operators.

To demonstrate a non-trivial ground state manifold that exists in the eigenstate space spanned by the above operators, we considered an interacting chain with next-nearest neighbors of the form

$$\sum_{i=1}^{N-1} \left( t\hat{H}_{KC}^{(0,i)} + U\hat{H}_{KC}^{(1,i)} \right) + t' \sum_{j=1}^{N-2} \hat{H}_{KC}^{(2,j)}. \tag{7}$$

Using DMRG on a length $N=12$ chain, we empirically determined that the Kitaev chain ground states $|\psi_{KC}^{\pm}\rangle$ are also degenerate ground states of Eq. (7) for $t>0$ and $U/t \gtrsim 2[(t'/t)^2 - 1]$. At $t'=0$, this model corresponds to a previously discovered interacting Kitaev chain model described by Ref. 2.

Many physically reasonable Hamiltonians on various lattice geometries, such as open square lattices, ladders, and cylinders, with interactions and anisotropy can be constructed from the operators in this space, all with the one-dimensional $|\psi_{KC}^{\pm}\rangle$ states as degenerate eigenstates and possibly many with them as ground states. For example, the Hamiltonian

$$\sum_{i=1}^{N/2-1} \left( t_{\parallel}\hat{H}_{KC}^{(0,2i)} + U_{\parallel}\hat{H}_{KC}^{(1,2i)} \right) + t_{=} \sum_{i=1}^{N/2-2} \hat{H}_{KC}^{(3,2i,2i+3)} + t_{\times} \sum_{j=1}^{N-2} \hat{H}_{KC}^{(2,j)}, \tag{8}$$

which is constructed from the above operators, forms a particular interacting two-leg ladder model that has the $|\psi_{KC}^{\pm}\rangle$ states as degenerate eigenstates.

### B. Heisenberg chain ground state

In this section, we discuss our results of using EHC to find new parent Hamiltonians for the ground state $|\psi_H\rangle$ of the Heisenberg chain: $\hat{H}_H = \sum_{n=1}^{N} \mathbf{S}_n \cdot \mathbf{S}_{n+1}$. The target space we provided as input to the EHC method was the same as for the XX chain discussed in the main paper, i.e., it was spanned by all possible two-site spin interactions of the form $\{S_n^x S_m^x, S_n^y S_m^y, S_n^z S_m^z\}$, where $S^x, S^y, S^z$ are spin-1/2 operators and $n, m = 1, \dots, N$. Applying the EHC method to an $N = 12$ length chain, we found an eigenstate space of $|\psi_H\rangle$ of dimension $3N + 3 = 39$. In this space we found $3N = 36$ operators related to conserved quantities, discussed in a later section. The three remaining Hamiltonians in this space are

$$\hat{H}_H^{(a)} = \sum_{n=1}^{N} f^a(n) \mathbf{S}_n \cdot \mathbf{S}_{n+1}, \tag{9}$$

where $f^a(n) = 1, \cos(2\pi n/N), \sin(2\pi n/N)$ for $a = 0, 1, 2$, respectively. The state $|\psi_H\rangle$ is a zero energy eigenstate of the sinusoidally modulated Hamiltonians $\hat{H}_H^{(1)}, \hat{H}_H^{(2)}$. Using DMRG, we studied the following Hamiltonians

$$\hat{H}_H + \alpha \hat{H}_H^{(1)} + \beta \hat{H}_H^{(2)}, \tag{10}$$

and empirically found that the $|\psi_H\rangle$ state is a ground state in the region $\alpha^2 + \beta^2 \leq 1$. We also verified numerically for small finite sizes that $\hat{H}_H, \hat{H}_H^{(1)}, \hat{H}_H^{(2)}$ all do not commute with one another.

### C. Majumdar-Ghosh model (singlet dimer) ground states

In this section, we discuss our DEHC results for the two degenerate singlet dimer state ground states $\left|\psi_{SD}^{\pm}\right\rangle$ of the Majumdar-Ghosh model. We used the same $d_T = 3N(N-1)/2 = 198$ dimensional target space as for the XX chain and Heisenberg chain ground state phase expansion results. Applying the EHC method to a chain of length $N = 12$, we found a large eigenstate space containing 108 "block" operators of the form

$$\hat{H}_{MG}^{(\rho,i,\nu)} = \sum_{j=1}^{2\nu-1} \sum_{k=j+1}^{2\nu} S_{i+j}^{\rho} S_{i+k}^{\rho} \tag{11}$$

for all sites $i$, where $\rho = x, y, z$ and $\nu = 1, \dots, N/4$. Ref. 3 showed that the singlet dimer states $\left|\psi_{SD}^{\pm}\right\rangle$ are ground states of the isotropic versions of these block operators,

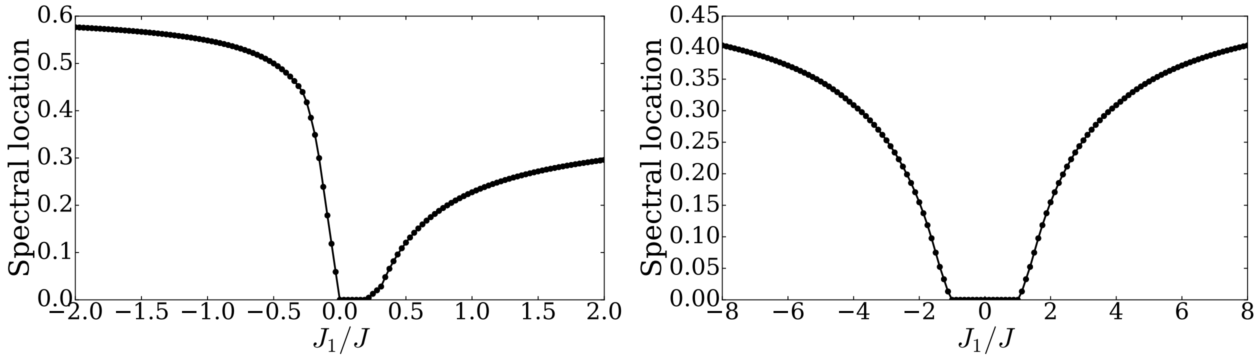


(a) (b)

FIG. S1. The spectral location of two target states for Hamiltonians found with EHC, calculated with ED for size $N = 12$ systems. The spectral location is defined as $(E_T - E_0)/(E_f - E_0)$, where $E_T$ is the target state energy, $E_0$ is the ground state energy, and $E_f$ is the largest energy eigenvalue of the Hamiltonian. Zero means that the target state is a ground state and one means that it is an anti-ground state. (a) The location of the UFI state $|\psi_{UFI}\rangle$ in the spectrum of the Hamiltonian $J\hat{H}_I + J_1(\hat{H}^{(1)}_{UFI} + \hat{H}^{(2)}_{UFI})$ with $J > 0$. (b) The location of the Heisenberg chain ground state $|\psi_H\rangle$ in the spectrum of the Hamiltonian $J\hat{H}_H + J_1\hat{H}^{(1)}_H$ with $J > 0$.

i.e., $\sum_\rho \hat{H}^{(\rho,i,\nu)}_{MG}$, and that the isotropic block operators do not commute with the Majumdar-Ghosh model $\hat{H}_{MG}$.

This large eigenstate space is consistent with the fact that $\hat{H}_{MG} = \frac{1}{2}\sum_{i=1}^{N}\sum_{\rho=x,y,z}\hat{H}^{(\rho,i,1)}_{MG}$ is frustration-free. Due to the frustration-free nature of the Majumdar-Ghosh model, the target states $\left|\psi^{\pm}_{SD}\right\rangle$ are also the degenerate ground states of a large family of Hamiltonians constructed from these local operators. The eigenstate space of models discussed in the state collision example in the main paper is a specific example of Hamiltonians which can be constructed from these "block operators."

## IV. ENERGETICS AND DEGENERACY OF TARGET STATES IN EHC

While the EHC method is able to find Hamiltonians with the target state $|\psi_T\rangle$ as an eigenstate, it is not able to guarantee that the target state is a ground state of these Hamiltonians. In fact, as we discuss in the main paper, $|\psi_T\rangle$ only remains in the ground state manifold of the eigenstate space Hamiltonians for certain ranges of parameters and is oth-

erwise an excited state. One scenario for an eigenstate is that it is low in the spectrum. In such situations, the physics of this eigenstate is potentially important at finite temperature or when excitations are probed experimentally. Alternatively, low-lying eigenstates may suggest a nearby level crossing with the ground state (implying the existence of a nearby phase) or indicate one sector of a topologically degenerate system.

Another scenario is that the eigenstate might be high in the spectrum. In the case of non-degenerate area (or log) law eigenstates, this would be a violation of the eigenstate thermalization hypothesis (ETH). Alternatively the eigenstate might be area-law but degenerate with other eigenstates, which does not directly violate ETH since there might be a purification of the degenerate space in which the degenerate states are volume-law. Eigenstate degeneracy is independently interesting, since generically we expect that level repulsion would prevent such degeneracy, and could indicate additional local integrals of motion.

Fig. S1 shows two examples of the spectral locations of target states for Hamiltonians constructed in the Hamiltonian discovery of the UFI model and in the phase expansion of the Heisenberg model. We find that while in some parameter regimes it is a ground state, in others it is an eigenstate high in the spectrum. For $|\psi_{UFI}\rangle$, we find that, in the parameters considered in Fig. S1(a), the eigenstate is linearly degenerate allowing for its location high in the spectrum. Interestingly, for $|\psi_H\rangle$, shown in Fig. S1(b), we find that the state is the unique eigenstate in spite of its location in the spectrum, suggesting a violation of ETH.

We also consider the degeneracy of other operators in the eigenstate space. For $\hat{H}^{(2)}_{UFI}$ on an $N = 12$ site ladder, the uniform frustrated Ising state $|\psi_{UFI}\rangle$ is a zero energy eigenstate in a degenerate subspace consisting of 124 degenerate eigenstates; for the Hamiltonian $\hat{H}^{(1)}_{H}$ on a $N = 12$ site chain, the $|\psi_H\rangle$ state is a zero energy eigenstate in a degenerate subspace of 260 eigenstates. However, it is important to note that such eigenstate degeneracy can be dramatically modified by adding other Hamiltonians in the eigenstate space. For example, the random Hamiltonian $\hat{H}_I - 0.03\hat{H}^{(1)}_{UFI} + 1.31\hat{H}^{(2)}_{UFI}$ on $N = 12$ sites has $|\psi_{UFI}\rangle$ as one of 8 degenerate excited states; in a more extreme example, the Hamiltonian $\hat{H}_H + \alpha\hat{H}^{(1)}_{H}$ for most $\alpha$ has the state $|\psi_H\rangle$ as a unique eigenstate.

## V. CONSTRUCTED HAMILTONIANS AND CONSERVED QUANTITIES

In our phase expansion results for the XX and Heisenberg chains of length $N = 12$, we encountered non-local operators in our eigenstate space that are related to conserved quantities.

For example, the XX chain Hamiltonian $\hat{H}_{XX} = \sum_{n=1}^{N}(S_n^x S_{n+1}^x + S_n^y S_{n+1}^y)$ commutes with the total $S^z$ operator, $S_{tot}^z \equiv \sum_{n=1}^{N} S_n^z$. Since the target space we considered for the phase expansion of the XX chain contains only two-site interactions, $S_n^\rho S_m^\rho$, the total $S^z$ operator itself is not in the target space. However, from our results, we found that the eigenstate space contained $N$ operators related to $S_{tot}^z$ of the following form

$$\hat{H}_z^{(n_0)} = \sum_{n \neq n_0} S_{n_0}^z S_n^z = S_{n_0}^z (S_{tot}^z - S_{n_0}^z) = S_{n_0}^z S_{tot}^z - 1/4 \tag{12}$$

where $n_0 = 1, \ldots, N$. These operators connect a single site $n_0$ with all other sites on the chain through an Ising spin-spin interaction. Since $S_{tot}^z |\psi_{XX}\rangle = 0$ for even length spin chains, $|\psi_{XX}\rangle$ is an eigenstate of all $\hat{H}_z^{(n_0)}$ operators with eigenvalue $-1/4$ when $N$ is even. Despite the fact that $[\hat{H}_{XX}, S_{tot}^z] = 0$, the related $\hat{H}_z^{(n_0)}$ operators do not commute with $\hat{H}_{XX}$, which we checked numerically for small finite-size chains. Interestingly, the operator $(S_{tot}^z)^2$, which does commute with $\hat{H}_{XX}$, can be constructed as a linear combination of the $\hat{H}_z^{(n_0)}$ operators.

For the Heisenberg chain, we found a similar situation for even $N$ chains. Namely, there are $3N$ operators of the form $\hat{H}_\rho^{(n_0)} \equiv \sum_{n \neq n_0} S_{n_0}^\rho S_n^\rho$ for $\rho = x, y, z$ in the eigenstate space of $|\psi_H\rangle$. The Heisenberg chain ground state $|\psi_H\rangle$ is also an eigenstate of $\hat{H}_\rho^{(n_0)}$ with eigenvalue $-1/4$. We also numerically determined that the $\hat{H}_\rho^{(n_0)}$ operators do not commute with $\hat{H}_H$ for small finite-size chains.

## VI. BOUNDARY CONDITION AND FINITE-SIZE EFFECTS WITH CONSTRUCTED HAMILTONIANS

For our phase expansion calculations of the XX chain and Heisenberg chain, we found different parent Hamiltonians when the boundary conditions used to define the target state $|\psi_T\rangle$ were open instead of periodic. For example, we used the EHC method to construct parent Hamiltonians for $|\psi_{oH}\rangle$, the ground state of the open Heisenberg chain. For this

target state and the same target space as considered in the periodic case, we found only two operators in the eigenstate space

$$\hat{H}_{oH}^{(c)} = \sum_{n=1}^{N-1} h^c(n)\mathbf{S}_n \cdot \mathbf{S}_{n+1}, \tag{13}$$

where $h^c(n) = 1, \sin(\pi(n - N/2)/(N+1))$ for $c = 0, 1$. Likewise, we used the EHC method to construct parent Hamiltonians for $|\psi_{oXX}\rangle$, the ground state of the open XX chain, and found the reduced eigenstate space of operators

$$\hat{H}_{oXX}^{(d,\epsilon)} = \sum_{n=1}^{N-1} \epsilon^n r^d(n) \left(S_n^x S_{n+1}^x + \epsilon S_n^y S_{n+1}^y\right) \tag{14}$$

where $\epsilon = \pm 1$, and $r^d(n) = 1, \sin(\pi(n - N/2)/(N+1))$ for $d = 0, 1$. In both cases, two full-period sinusoidally modulated Hamiltonians were replaced by a single half-period sinusoidally modulated Hamiltonian centered at the bond between sites $N/2$ and $N/2+1$.

Finally, when applying the EHC method to the periodic XX chain ground state $|\psi_{XX}\rangle$, we found four operators in our eigenstate space of the form

$$\hat{H}_{XX}^{(k)} = \sum_{n=1}^{N} u^k(n) \left(S_n^x S_{n+1}^x + S_n^y S_{n+1}^y\right) + \sum_{n=1}^{N} \sum_{r=1}^{N-1} v^k(n,r) S_n^z S_{n+r}^z \tag{15}$$

where $k = 0, 1, 2, 3$ and

$$\begin{aligned}
u^0(n) &= \sin\left(\frac{4\pi}{N}n + \frac{3\pi}{N}\right) & v^0(n,r) &= +2\sin(\pi/N)\sin\left(\frac{4\pi}{N}(n-1) + \frac{2\pi}{N}r\right) \\
u^1(n) &= \cos\left(\frac{4\pi}{N}n + \frac{3\pi}{N}\right) & v^1(n,r) &= +2\sin(\pi/N)\cos\left(\frac{4\pi}{N}(n-1) + \frac{2\pi}{N}r\right) \\
u^2(n) &= \sin\left(\frac{6\pi}{N}n + \frac{9\pi}{N}\right) & v^2(n,r) &= +\cos\left(\frac{\pi}{N}r\right)\cos\left(\frac{6\pi}{N}(n-1) + \frac{3\pi}{N}r\right) \\
u^3(n) &= \cos\left(\frac{6\pi}{N}n + \frac{9\pi}{N}\right) & v^3(n,r) &= -\cos\left(\frac{\pi}{N}r\right)\sin\left(\frac{6\pi}{N}(n-1) + \frac{3\pi}{N}r\right)
\end{aligned}$$

We believe that these operators, which contain sinusoidally modulated nearest neighbor XX interactions as well as sinusoidally modulated long-range Ising interactions, are related to finite-size effects on the $N = 12$ chain.

[1] A. Y. Kitaev, "Unpaired Majorana fermions in quantum wires," Phys. Usp. **44**, 131 (2001).

[2] H. Katsura, D. Schuricht, and M. Takahashi, "Exact ground states and topological order in interacting Kitaev/Majorana chains," Phys. Rev. B **92**, 115137 (2015).

[3] B. Kumar, "Quantum spin models with exact dimer ground states," Phys. Rev. B **66**, 024406 (2002).
